# Supplementary material for: Kolmogorovian turbulence in transitional pipe flows
Source: arXiv:1701.04048 ancillary file (2017-01-15)
Supplement: Supplementary file 1 [file flashes_supp_mat.pdf]

# Supplemental Material:
# Kolmogorovian turbulence in transitional pipe flows

## 1 Methods

**Experimental setup.** Our experimental setup is similar to other transition pipe experiments in which the flow is driven by gravity (see, e.g., [1, 2]). Fig. S-1 shows a schematic of the setup. The pipe is 20 m long, made of 1 m-long cylindrical glass tubes of inner diameter D = 2.5 cm ± 10$\mu$m. The tubes are aligned using a laser level and connected using acrylic connectors, which also have an inner diameter of 2.5 cm ± 10 $\mu$m. Several of these connectors have a pair of diametrically-opposite holes (of diameter 1 mm), which serve as pressure taps or as a syringe tap.

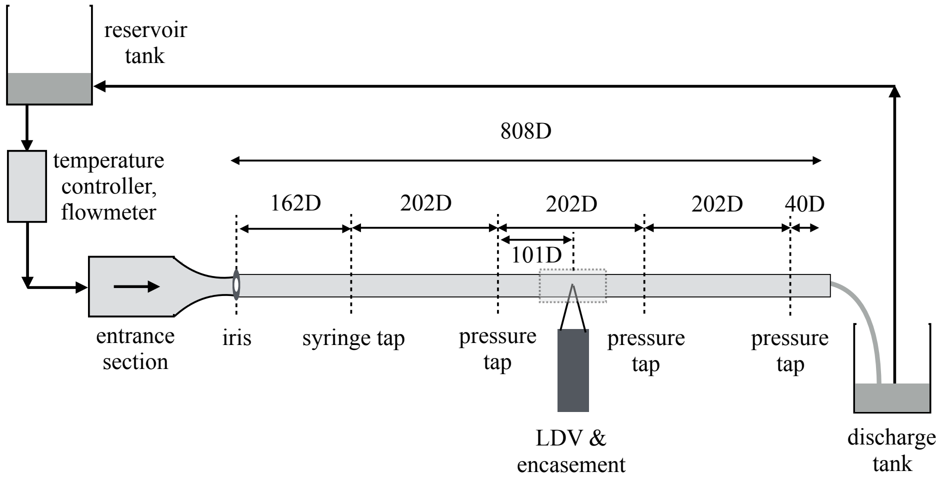


Figure S-1: Schematic of the experimental setup. The arrows indicate the direction of the recirculating flow. For transitional flows with puffs, we use the two pressure taps closest to the laser Doppler velocimeter (LDV) to measure the pressure drop over a lengthspan of 202$D$; see Fig. S-2. For laminar flows, transitional flows with slugs, and turbulent flows, we use all the pressure taps to measure the pressure drop over lengthspans of 202$D$ and 404$D$.

The starting point for the flow is a large reservoir tank which stores water at a constant pressure head. The reservoir tank sits on an elevator whose height we adjust to set a pressure drop for the flow. In addition, we use a ball valve at the exit of the reservoir to further control the flow rate.

After exiting the reservoir, the water passes through a flexible hose to a heat exchanger that is coupled with a Julabo temperature bath. This fixes the temperature of the water to the room temperature, 23 ± 0.1 °C. Thereafter, the water passes through a Yokogawa magnetic flowmeter,

which we use to measure the time series of flow rate through the pipe, $Q(t) = \pi(D/2)^2U(t)$. The time series of Reynolds number is defined as $Re(t) = DU(t)/\nu$, where $\nu = 0.009344$ cm$^2$/s is the kinematic viscosity of water at 23 °C. We average $Re(t)$ over long time to get $Re$.

Another flexible hose connects to the pipe's entrance section. The entrance section consists of several stages of obstacles (to homogenize the flow and to damp out perturbations) and a bell-shaped flow-conditioning section (to enable a smooth entrance to the pipe). The obstacles consist of one honeycomb lattice and two meshes situated several cm apart. Using several bleed holes located at the top of the entrance section we remove any air bubbles from the water. After passing through the flow-conditioning section, the water enters the pipe.

The largest pressure drop occurs in the segments before the pipe, so that the fluctuations in $Re$ during the transition are typically $< 1\%$. At the end of the pipe the water exits into a discharge tank. We pump the water back to the reservoir tank, completing the flow circuit. The gravity-driven flow remains laminar till the highest $Re$ we have tested, $Re \approx 8300$. For the turbulent flow data shown in Fig. 3 in the manuscript, we increased the highest $Re$ to $\approx 14,000$ using a pump.

See Supplementary Text for a discussion of pressure-drop measurements ($\Delta P(t)$), velocity measurements (axial and radial velocities at the centerline, $u(t)$ and $v(t)$, respectively), and perturbations to induce transition (iris and syringe pumps).

**Computing $f$ for puffs.** Owing to its size ($\sim 20D$), a single puff cannot span the lengthspan $\Delta L = 202D$ over which we measure pressure drop. This presents two problems. First, the contribution of a single puff to the pressure drop $\Delta P(t)$ measured over $\Delta L$ is small, and second, the value of $\Delta P(t)$ reflects the combined contribution of the puff and the laminar plug spanning the remaining $\sim 9/10$ of $\Delta L$. In order to increase the contribution from the puffs, we use syringe pumps to create a train of equi-spaced puffs (Fig. S-2a). Consequently, several puffs contribute to $\Delta P(t)$ at any time.

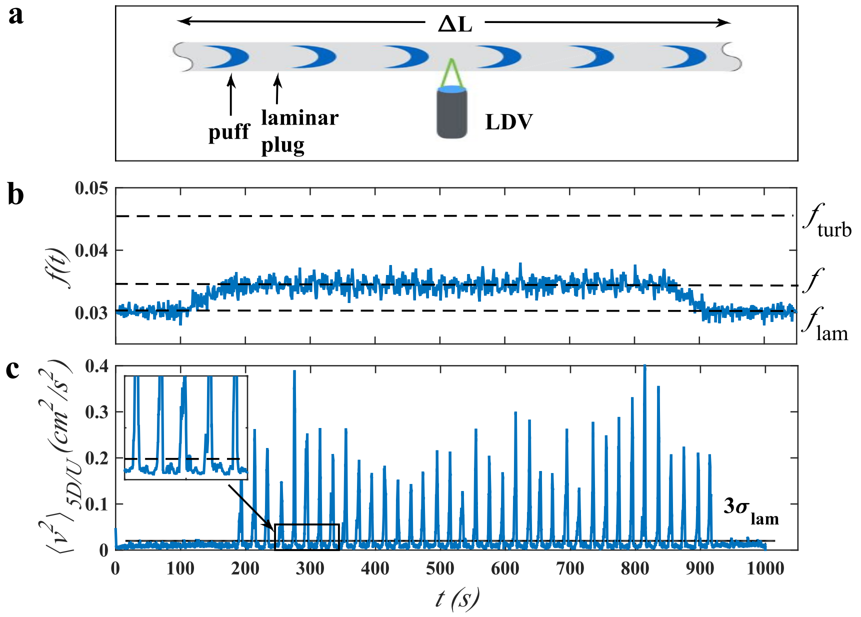


Figure S-2: Computing $f$ for puffs, $f_{\text{puffs}}$. (a) Schematic of the section (of lengthspan $\Delta L = 202D$) where we measure the pressure drop for a train of puffs (sketched in the figure). The LDV stationed at the middle of this section measures the time series of the radial velocity at the centerline, $v(t)$. We also simultaneously measure the time series of pressure drop $\Delta P(t)$ and mean velocity $U(t)$. (b) Sample time series $f(t)$ for a train of about 30 puffs. We compute $f(t)$ using $\Delta P(t)$ and $U(t)$. $f$ is the time-averaged $f(t)$ for the train of puffs, with 6-7 puffs concurrently present in $\Delta L$. For reference, we mark $f_{\text{lam}}$ and $f_{\text{turb}}$ at the flow $Re$. (c) Attendant to panel (b), simultaneous measurements of the smoothed $\langle v(t)^2\rangle_{5D/U}$, which we use to determine $\gamma$. We mark the threshold deviation $\delta = 3\sigma_{lam}$. (Inset: zoomed-in view.) The puffs correspond to $\langle v^2(t)\rangle_{5D/U} \geq \delta$.

The time series of friction, $f(t)$, for the train of puffs fluctuates about $f$ for $t > 500$ s ($> 2000$ $D/U$); see Fig. S-2b. $f$ is set by the combined contribution of the puffs and the intervening laminar plugs. We separate the contributions, as in transitional boundary layers [3], and write $f$ as a weighted average:

$$f = \gamma f_{\text{puffs}} + (1-\gamma) f_{\text{lam}}, \quad (1)$$

where $f_{\text{puffs}}$ is the $f$ for puffs, $\gamma$ is the intermittency factor (the fraction of the flow spanned by the puffs), and $f_{\text{lam}}$ is the $f$ for laminar plugs. Once we deduce $\gamma$ (see below), we use the experimentally determined $f_{\text{lam}}$ (from the laminar flow before and after the train of puffs; here we have assumed that the $f$ for the laminar plugs equals that for the laminar flow before and after the train of puffs)

and solve for $f_{\mathrm{puffs}}$.

To determine $\gamma$, we measure the time series of axial velocity at the centerline, $v(t)$, and use a thresholding method similar to [4, 5, 6, 7, 8]. In this method, to disentangle the puffs from the laminar plugs, a non-negative indicator function $I(t)$ is invoked so that:

$$\text{the flow at time } t \in \begin{cases} \text{laminar, if } I(t) < \delta + I_{\mathrm{lam}} \\ \text{puff, if } I(t) \geq \delta + I_{\mathrm{lam}}, \end{cases} \tag{2}$$

where $I_{\mathrm{lam}}$ is the mean value of $I(t)$ for the laminar plugs and $\delta$ is the allowed threshold of deviation from this value. (This approach can also be used to disentangle slugs from laminar plugs.) Previous work [4, 5, 6, 7, 8] adopted various definitions for $I(t)$: the squared in-plane velocity, the squared vorticity, the light intensity—all averaged over a spatial extent of the flow (in order to push its mean above the laminar mean of zero). Using our single-point measurement of $v(t)$, we compute $v^2(t)$ and perform an analog of averaging over a spatial extent—we smooth the time series $v^2(t)$ with a window of fixed size $T = 5D/U$; the resultant $\langle v^2(t)\rangle_{5D/U}$ is our choice for $I(t)$. This moving average, while quite simple, is in fact optimal for the task of reducing noise and enhancing step response [9], allowing us to cleanly identify the puffs.

To determine $\gamma$ from $I(t)$, we need to consider the threshold deviation $\delta$. To that end, we measure the smoothed $\langle v^2(t)\rangle_{5D/U}$ for the laminar flow before and after the train of puffs, and compute its probability distribution (which includes instrumental and experimental noise). From this distribution, which is approximately Gaussian, we use the typical three standard deviations as our threshold deviation, $\delta = 3\sigma_{\mathrm{lam}}$, away from the mean value $I_{\mathrm{lam}} = \langle v^2\rangle_{\mathrm{lam}} \approx 0$. In Fig. S-2c, we show an example of $\langle v^2(t)\rangle_{5D/U}$ for a train of puffs. The puffs correspond to $\langle v^2(t)\rangle_{5D/U} \geq \delta$ and the fraction of $t$ where this equation holds yields $\gamma$.

Our estimate of $\gamma$ is affected by the choice of the smoothing window size $T$ and the threshold deviation $\delta$. This, in turn, affects the value of $f_{\mathrm{puffs}}$. The variation in $f_{\mathrm{puffs}}$ is $\approx 6\%$ if we double the window size from $5D/U$ to $10D/U$. (Note that the upper limit of $T$ is $\sim 20D/U$, the time it would take a puff to traverse the measurement point.) The variation in $f_{\mathrm{puffs}}$ is $< 5\%$ if we used $\delta = 2\sigma_{\mathrm{lam}}$ or $4\sigma_{\mathrm{lam}}$ instead of $3\sigma_{\mathrm{lam}}$. For additional discussion, see Supplementary Text.

**Computing $E(k)$ and $\eta$.** For puff flows, slug flows, and turbulent flows in our experiments, we compute the (one-dimensional) turbulent-energy spectra $E(k)$ using the time series of axial and radial velocities, $u(t)$ and $v(t)$, respectively. For the transitional flows, $u(t)$ and $v(t)$ include contributions from the laminar plugs and the flashes. To disentangle $u(t)$ and $v(t)$ corresponding to the flash flows, we use the thresholding method described previously.

Assuming Taylor's frozen turbulence hypothesis [10], we compute the axial $E(k)$ from $u(t)$ and the radial $E(k)$ from $v(t)$. For puff flow and slug flow, we note that the high $k$ region of the axial and radial $E(k)$ collapse on the same curve (Fig. S-3), signifying isotropy of high $k$, i.e., small-scale isotropy. For isotropic turbulence, we can use the axial $E(k)$ to compute the viscous lengthscale $\eta$ as [10]

$$\eta = \left( \frac{\nu^3}{15\nu \int_0^\infty k^2 E(k) dk} \right)^{1/4}, \tag{3}$$

where the denominator is the turbulent power $\varepsilon$ and $15\nu k^2 E(k)$ is the dissipation spectrum. Plotting the dissipation spectrum reveals that the entire dissipative range of $E(k)$ is not resolved in our LDV measurements (see Fig. S-4). The region at the highest $k$ is not trustworthy because it is influenced by the intermittent sampling time of the LDV at these higher wavenumbers (frequencies) [11, 12]. We define a cutoff $k$ (above which we do not trust the spectra) as the $k$ where $k^2E(k)$ exhibits an inflection point (see the dotted line in Fig. S-4). To estimate the contribution of the unresolved scales to computing the integral in Eq. (3), we tested three methods: (1) we used the exponential model, $k^{5/3}E(k) \propto e^{-Ak}$, in the dissipative range [10]; (2) we used the Pao model, $k^{5/3}E(k) \propto e^{-Bk^{4/3}}$, in the dissipative range [10]; and (3) we simply chopped off $E(k)$ at the cutoff $k$. (The constants $A$ and $B$ are fitting parameters, which we determine separately for each measurement.) The $\eta$ determined by all three methods agrees within 5%. We used the exponential model for the data shown in Fig. 3 of the manuscript. For further discussion, see Supplementary Text.

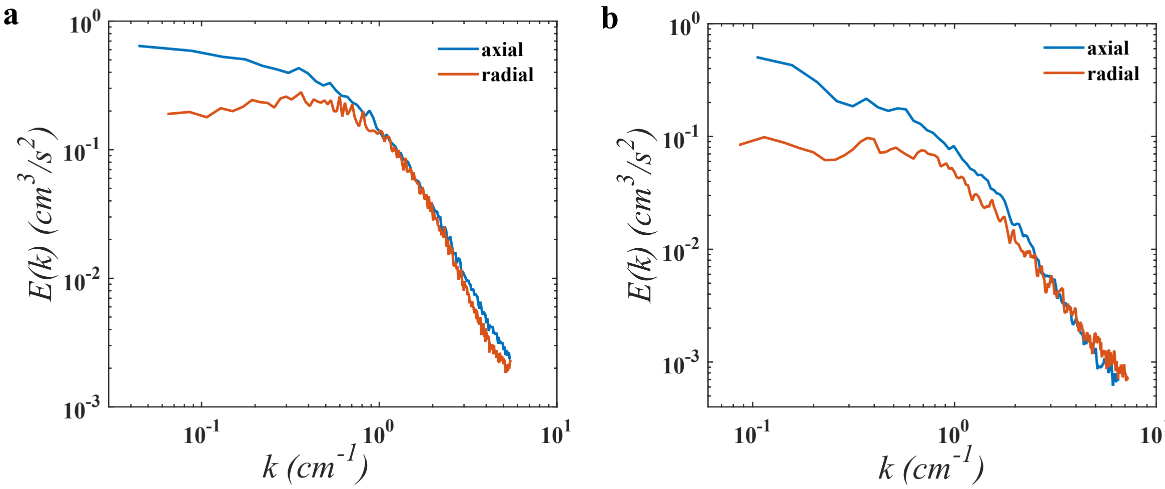


Figure S-3: Example of axial $E(k)$ and radial $E(k)$ for (a) slug flow ($Re \approx 4200$) and (b) puff flow ($Re \approx 2150$). At high $k$, the $E(k)$ exhibit small-scale isotropy.

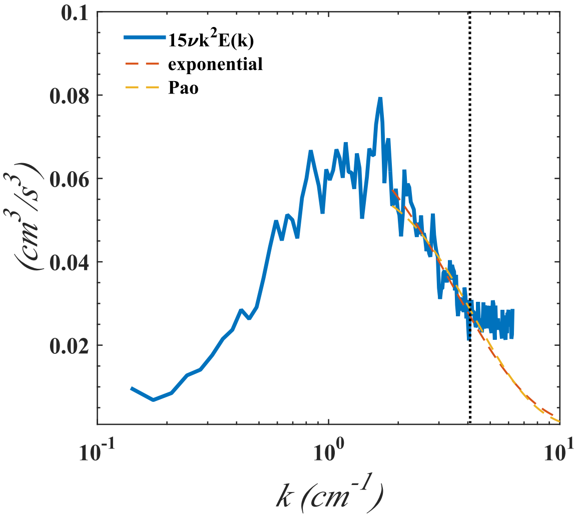


Figure S-4: Example of the dissipation spectrum, $15\nu k^2 E(k)$, for puff flow ($Re \approx 2300$). The dotted line indicates the cutoff $k$. We also show the exponential model and the Pao model (dashed lines), which we use to extend the spectrum beyond the cutoff $k$.

# 2 Supplementary Text

**A note on the unitless pressure drop in Reynolds's 1883 paper.** In the manuscript we noted that the fluid friction $f$, a unitless measure of pressure drop per unit length of pipe, is defined as

$$f \equiv \frac{D\Delta P/\Delta L}{\rho U^2/2}, \tag{4}$$

where $D$ is the diameter of the pipe, $\Delta P/\Delta L$ is the pressure drop per unit length of pipe, $\rho$ is the density of the fluid, and $U$ is the mean velocity of the flow. Reynolds [13] used a different measure for unitless pressure drop, which can be expressed as

$$f_{\text{Reynolds}} \equiv \frac{D^3\Delta P/\Delta L}{\rho \nu^2}, \tag{5}$$

where $\nu$ is the kinematic viscosity of the fluid. Comparing $f$ and $f_{\text{Reynolds}}$, we note that

$$f_{\text{Reynolds}} = \frac{f Re^2}{2}, \tag{6}$$

where $Re$ is the Reynolds number, $Re \equiv UD/\nu$.

Fitting his experimental data for turbulent flows, Reynolds found $f_{\text{Reynolds}}(Re) \propto Re^{1.723}$, which from Eq. 6, corresponds to $f(Re) \propto Re^{-0.277}$, close to the Blasius law $f_{\text{turb}}(Re) \propto Re^{-1/4}$.

**Pressure-drop measurements.** The pipe in our experiments has three pressure taps (see Fig. S-1). The $f(t)$ and $f$ reported in the manuscript are computed using the pressure drop $\Delta P(t)$ measured between the first two pressure taps. Further, we simultaneously measure the pressure drop between the first and third pressure taps, and between the second and third pressure taps. The values of the pressure gradients from these measurements are within the error bars. The pressure drops are measured using Validyne low pressure differential pressure transducers (models DP103 and DP45) and a 35mbar NicheSensor pressure transducer. We calibrate the pressure transducers in situ with laminar flow as a reference. (We also cross-check the calibration using a hydrostatic head of water.) In Fig. S-5 we show a typical calibration curve. We record $\Delta P(t)$ and flow rate $Q(t)$ simultaneously on a computer at 1 Hz, where each point has been averaged over 1 s. From this data we determine $f(t) = \frac{D\Delta P(t)/L}{\frac{1}{2}\rho U(t)^2}$ and $Re(t)$ simultaneously.

Consider the error bars in $f$ (see Fig. 2 in the manuscript). The error bars are a combination of the intrinsic uncertainty of the instrument, the statistical uncertainty, and the calibration uncertainty. The DP103 has a rated 0.25% accuracy at full scale. With the Number 14 diaphragm, which has a 2206.5 barye range, this corresponds to a 5.52 barye uncertainty. The corresponding friction factor uncertainty $\delta f = f \times (\delta(\Delta P)/\Delta P)$ will depend on $Re$, typically being larger for lower $Re$. As an example, this intrinsic uncertainty for laminar flow at $Re = 1800$ is $\delta f = 0.00097$ ($f = 0.0351$), while for $Re = 3790$ it is $\delta f = 0.00024$ ($f = 0.0172$). The uncertainty from the calibration and the statistical uncertainty are of the same order of magnitude and at their largest relative value (for puffs) they all combine to $< 3\%$ of the determined value. We also calculated contributions to the uncertainty in $f$ from the fluctuations in $U(t)$, but found this uncertainty to be negligible.

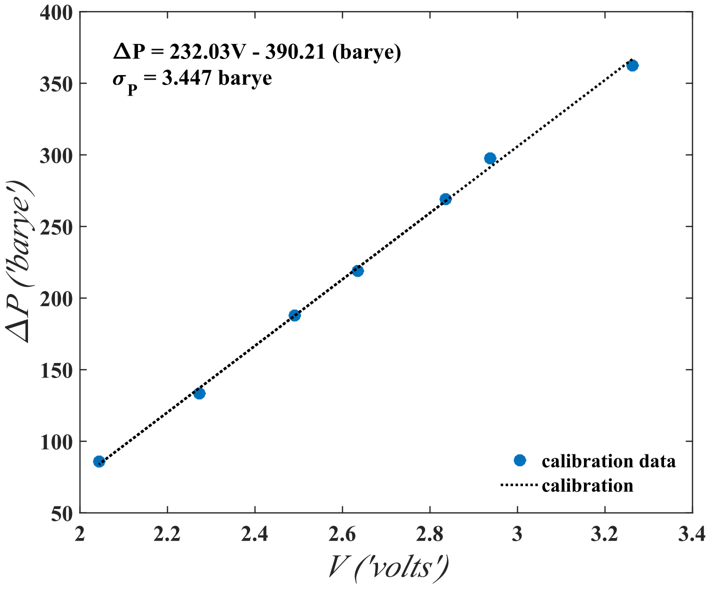


Figure S-5: Typical calibration curve, pressure drop vs. voltage ($\Delta P$ vs. $V$), for DP103. The flow is laminar ($Re \approx 800$ to $Re \approx 3500$). Using the laminar flow result $f_{\mathrm{lam}}(Re) = 64/Re$, we compute $\Delta P$ (dots), to which we fit a line to get the calibration curve (dotted line). We use the variation about the calibration curve to estimate the contribution from the calibration to the uncertainty in $f$.

**Velocity Measurements.** We use laser Doppler velocimetry (LDV, Dantec FiberFlow) to measure a time series of the axial velocity and radial velocity at the centerline of the pipe, $u(t)$ and $v(t)$, respectively. The LDV is stationed at the middle of the section of the pipe between the first two pressure taps (see Fig. S-1). At this location the pipe is housed inside a rectangular acrylic encasement filled with water—this is to reduce optical distortion; see Fig. S-6a. (This design is similar to [14].) Despite the optical encasement, there is still a small correction to $v(t)$, which, via ray tracing [15], we estimate to be $\approx 1.1909 v_{\text{measured}}(t)$. We seed the water in the pipe with small, 10 $\mu$m silver-coated, density matched particles. The data rate is usually $> 300$ Hz and the length of the time series is typically $\approx 1000$ s.

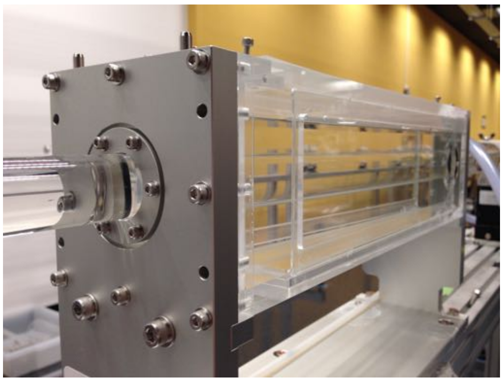

(a)

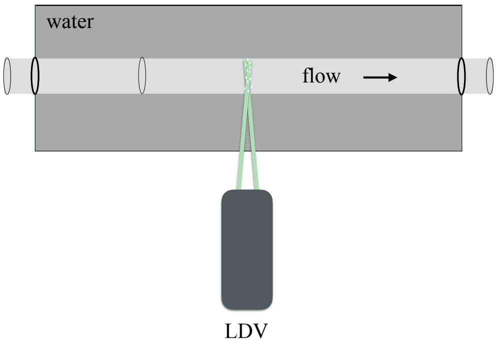


(b)

Figure S-6: (a) The acrylic encasement is filled with water and is used to reduce optical distortion due to the difference in refractive indices between glass, water, and air. (b) Schematic of the arrangement of LDV with the acrylic encasement. Because the measurement position is at the centerline of the pipe, the distortions are at their minimum.

**Perturbations.** The gravity-driven flow in our experiments remains laminar for all $Re$. (The highest $Re$ we can achieve for gravity-driven flow is $Re \approx 8300$.) In order to trigger turbulent flow, we employ two methods to perturb the flow. The first is an iris located at the entrance of the pipe, just after the flow conditioner. The iris has 16 stainless steel blades, which smoothly changes the size of the obstruction ($0 < h/R < 0.9$, where $h$ is the height of the obstruction). A frontal view of two iris positions is shown in Fig. S-7b, S-7c. With this iris we can smoothly adjust the $Re$ at which the flow transitions to turbulence [16]. In Fig. S-7a we plot $f$ vs. $Re$ for several $h/R$.

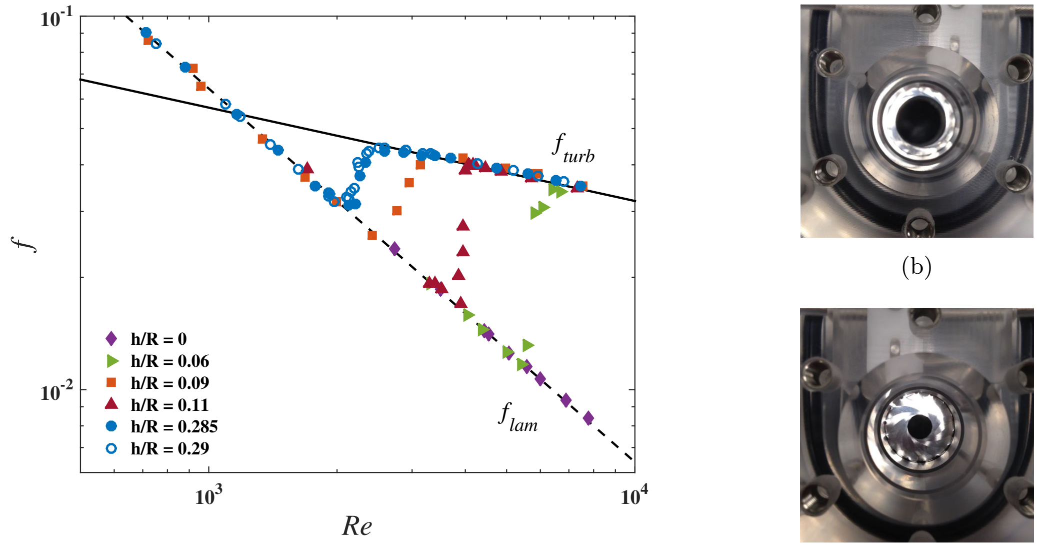


(a) (b) (c)

Figure S-7: (a) Example of $f$ vs $Re$ plots obtained by varying $h/R$. For $h/R = 0$, the flow is laminar. The larger the obstruction, the sooner the flow becomes turbulent. Photographs of iris openings of (b) $h/R \sim 0.28$ and (c) $h/R \sim 0.66$.

The second method we use to perturb the flow is by using two YMC YSP-201 syringe pumps connected to the holes of the syringe tap. We have used the pumps in two settings—(1) both inject water; (2) one injects and the other simultaneously withdraws the same mass of water—and have found no differences in the results [1, 2]. We typically inject (withdraw) the water for $< 1$s at a rate of 0.5 mL/s. This is $< 1\%$ of the pipe flow rate at $Re = 2000$ (and for larger $Re$ it is an even smaller percentage). The ratio of this injection flow rate to the pipe flow rate is a measure of the perturbation size, which must exceed a certain threshold to trigger turbulent flow [2]. This threshold decreases as $\propto 1/Re$ [2], which implies that once this threshold has been exceeded for a certain injection rate, the same injection rate can be used for all $Re$ to trigger turbulent flow.

**Computing $f$ for slugs and $f$ for puffs.** As discussed in the manuscript, determining $f$ for slugs is straightforward. In transitional flows with slugs, $p(f)$ is bimodal and $f(t)$ swings between $f_-$ (corresponding to the laminar plugs) and $f_+$ (corresponding to the slugs). (Using LDV measurements of $u(t)$ and $v(t)$, we have confirmed that the two regions of $f(t)$ correspond to the laminar plugs and the slugs.) The value of $f_-$ and $f_+$ can be determined either from the two peaks of $p(f)$ or by taking the average inside the span of time when $f(t)$ corresponds to the laminar plugs or to the slugs, respectively. In Fig. S-8 we show several typical plots of $f(t)$ and $p(f)$.

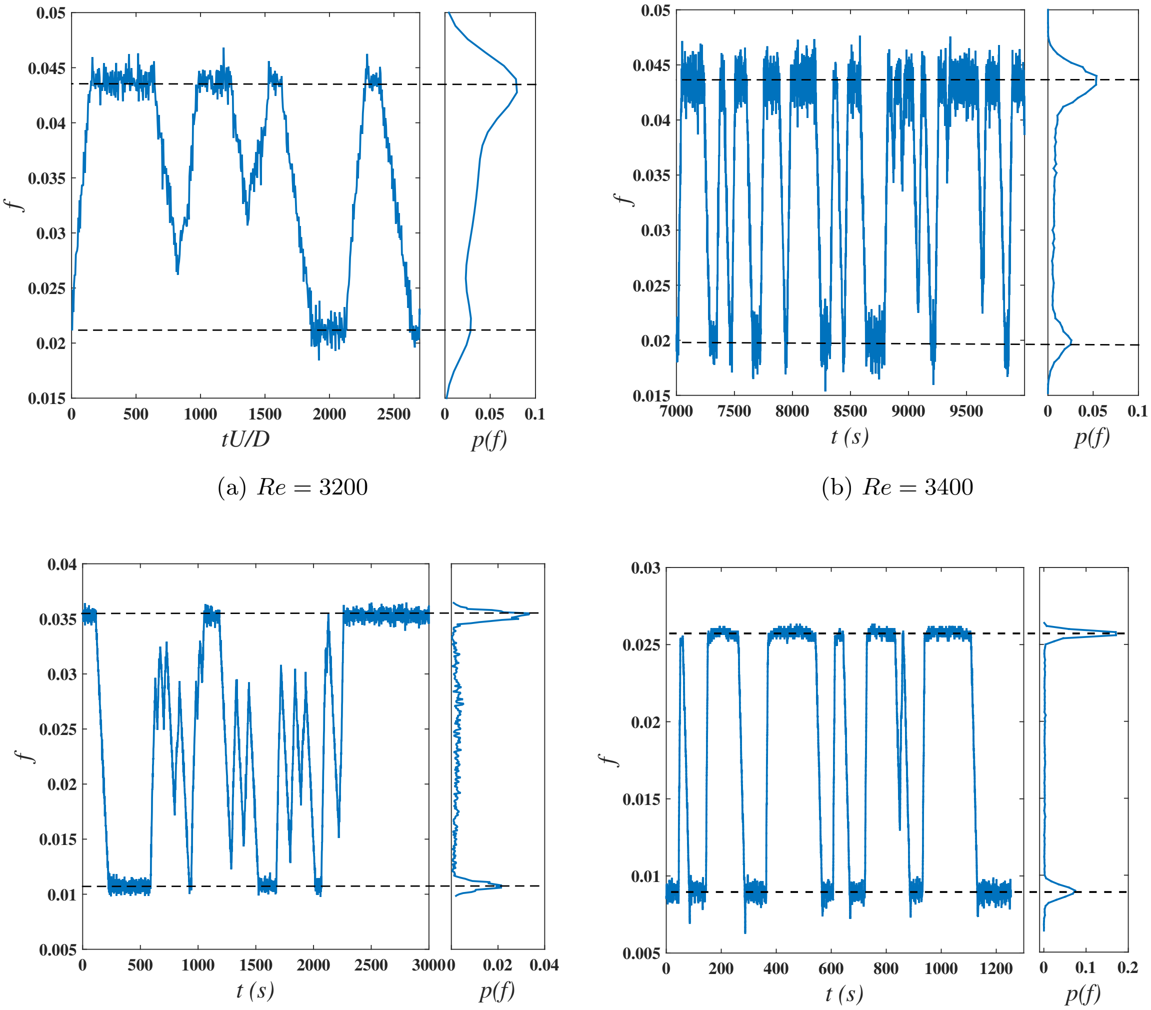


(a) $Re = 3200$ (b) $Re = 3400$ (c) $Re = 6200$ (d) $Re = 7500$

Figure S-8: Examples of $f(t)$ for transitional flows with slugs. We estimate the statistical uncertainty in $f$ from the standard deviation of the peaks in $p(f)$.

The puffs are much more limited in size than the slugs (typically $\approx 20D$ [2]), rendering the above approach ineffectual for puffs. As described in Methods, we adopt a different approach—we create

a train of puffs to establish a constant $f$ and determine $f$ for puffs, $f_{\text{puffs}}$, by solving Eq. 1:

$$f = \gamma f_{\text{puffs}} + (1 - \gamma) f_{\text{lam}}.$$

Here we discuss further details of computing the intermittency factor $\gamma$.

As a benchmark, we consider transitional flows with slugs for which we have determined $f$ for slugs, $f_{\text{slugs}}$, using the procedure described above. In Fig. S-9a we show an example of a transitional flow with slugs at $Re \approx 4000$, where we have simultaneously measured $f(t)$ and $v(t)$. From $v(t)$ we compute the smoothed $\langle v^2(t) \rangle_{5D/U}$. To determine $\gamma$, we vary the threshold $\delta = n\sigma_{\text{lam}}$, where $n$ is an integer and $\sigma_{\text{lam}}$ is the standard deviation of $\langle v^2(t) \rangle_{5D/U}$ for the laminar flow before and after the slug. Different values of $\delta$ yield different values of $\gamma$, which, via Eq. 1 (with $f_{\text{slugs}}$ substituted for $f_{\text{puffs}}$), yield different values of $f_{\text{slugs}}$. In Fig. S-9b we show how $\gamma$ and $f_{\text{slugs}}$ vary with $\delta$. For $n$ between 1 and 4, $f_{\text{slugs}}$ varies by $< 5\%$. Comparing with the $f_{\text{slugs}}$ obtained from $f(t)$, we note that $\delta = 3\sigma_{\text{lam}}$ is a good choice for the threshold.

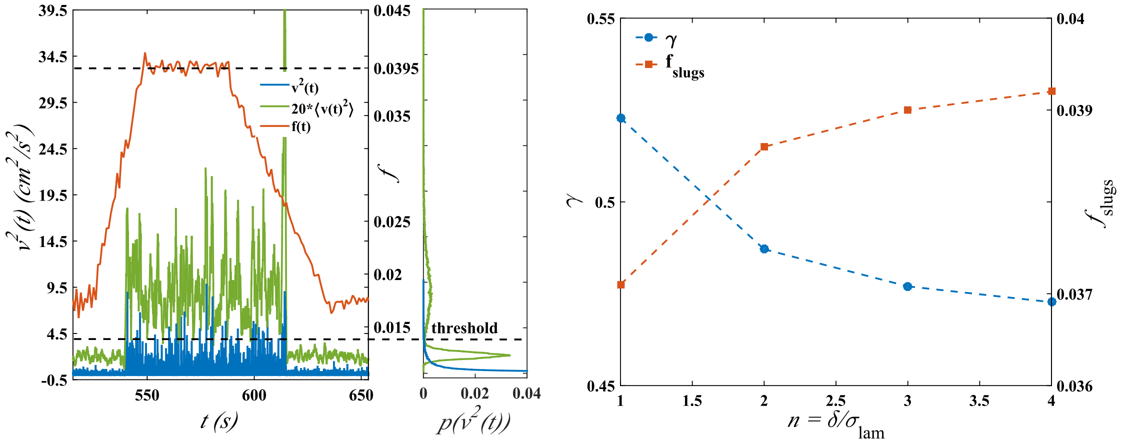


(a) (b)

Figure S-9: (a) Simultaneous measurement of $f(t)$ and $v^2(t)$ for a transitional flow with slugs at $Re \approx 4000$. From $f(t)$ we find that $f_{\text{slugs}} = 0.0395$. We also show the smoothed $\langle v^2(t) \rangle_{5D/U}$ (multiplied by 20 for clarity). Note that unlike $\langle v^2(t) \rangle_{5D/U}$, $v^2(t)$ can be zero for the slug flow. In the right panel we show the probability distribution functions of $v^2(t)$ and $\langle v^2(t) \rangle_{5D/U}$. The dashed line represents the threshold $\delta = 3\sigma_{\text{lam}}$. (b) $\gamma$ and $f_{\text{slugs}}$ as a function of $n = \delta/\sigma_{\text{lam}}$. $f_{\text{slugs}}$ varies by $< 5\%$.

Using the syringe pumps, we create a train of puffs, where we vary the frequency of injection from 1/10 to 1/30 Hz (Fig. S-10). (Our injection frequency is slower than the "optimal" frequency found by [17], so that there is no interference between the puffs.) Fig. S-11a shows $\langle v^2(t) \rangle_{5D/U}$ and Fig. S-11b shows the effect of varying the injection frequency and the threshold on $\gamma$ and $f_{\text{puffs}}$ (which we obtain from Eq. 1). The variation in $f_{\text{puffs}}$ is $< 3\%$. For the $f_{\text{puffs}}$ reported in Fig. 2 in the manuscript, we used $\delta = 3\sigma_{\text{lam}}$.

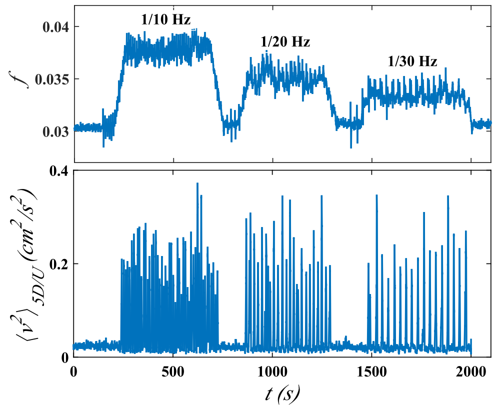


Figure S-10: An example of simultaneous $f(t)$ and $\langle v^2(t)\rangle_{5D/U}$ for trains of puffs (at $Re \approx 2300$) with three different injection frequencies $(1/10, 1/20$, and $1/30$ Hz).

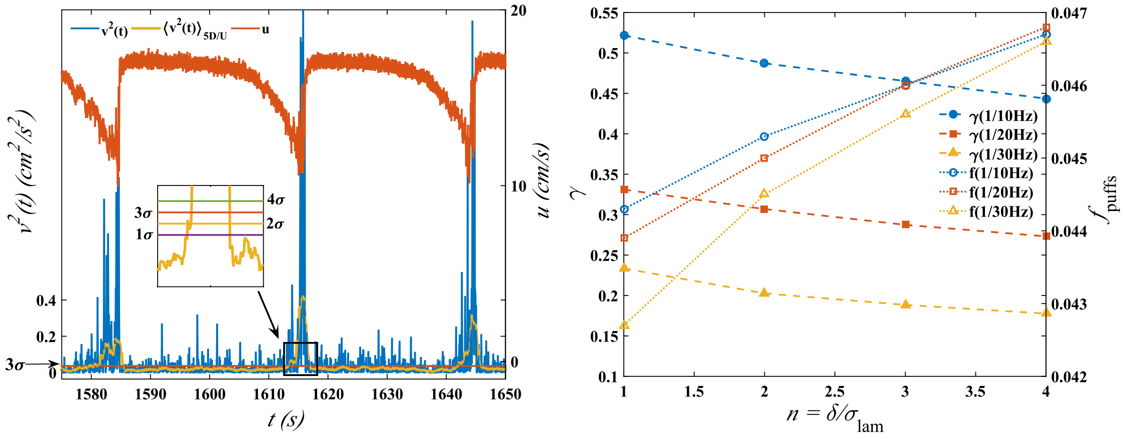


(a) (b)

Figure S-11: (a) A closeup view of $u(t)$, $v^2(t)$, and $\langle v^2(t)\rangle_{5D/U}$ for the train of puffs at injection frequency 1/30 Hz (see Fig. S-10). We mark the thresholds $\delta = n\sigma_{\mathrm{lam}}$. (b) $\gamma$ and $f_{\mathrm{puffs}}$ as a function of $n = \delta/\sigma_{\mathrm{lam}}$. $\gamma$ is necessarily distinct for different injection frequencies, but the variation in the resulting values of $f_{\mathrm{puffs}}$ is $< 3\%$ for the different frequencies and the choice of threshold.

**Computing $E(k)$ and $\eta$.** In Methods we have described the calculations of the turbulent-energy spectra $E(k)$ and the viscous lengthscale $\eta$. Here we supply additional details.

We identify the region of puff flow and slug flow using the threshold $\delta$. Just as with $f$, the value of $\eta$ may depend on the choice of $\delta$. In Fig. S-12 we show that this sensitivity to the choice of $\delta$ is small. Consistent with our choice of $\delta$ in computing $f_{\text{puffs}}$, we pick $\delta = 3\sigma_{\text{lam}}$ for computing $\eta$ for the puff flows and slug flows shown in Fig. 3 in the manuscript.

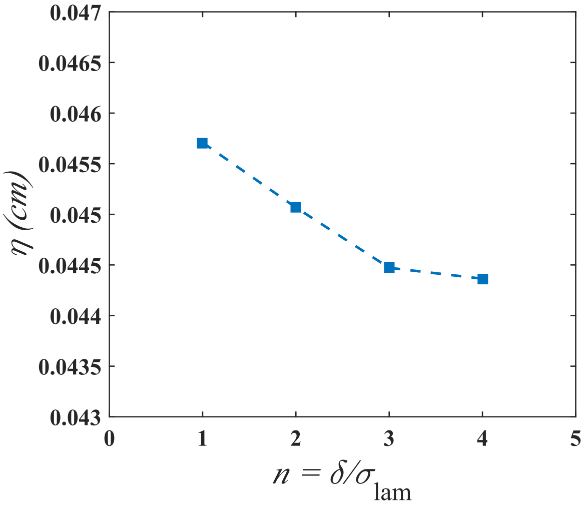


Figure S-12: Example of the effect of the threshold ($n = \delta/\sigma_{\text{lam}}$) on $\eta$ for a puff flow at $Re \approx 2300$. The resulting variation is $< 2\%$ in $\eta$.

Next we discuss the dissipative range of $E(k)$. As noted in Methods, because of the intermittent sampling time of LDV, the dissipative range for $E(k)$ above a cutoff $k$ is not trustworthy (see Fig. S-13). To extend $E(k)$ beyond the cutoff $k$ we have used two well-known models for the dissipative range—the exponential model ($k^{5/3}E(k) \propto e^{-Ak}$) and the Pao model ($k^{5/3}E(k) \propto e^{-Bk^{4/3}}$) [10]. In Figs. S-14a, S-14b we plot the premultiplied spectra $k^{5/3}E(k)$, which show a long linear region in a linear-log plot, indicating that the exponential model is a good fit. For each $Re$, we fit the exponential model or the Pao model to the region between the peak of $k^{5/3}E(k)$ and the cutoff $k$ and get the model constants $A$ or $B$, respectively. In Figs. S-14c, S-14d we show the exponential model and the Pao model extensions to the dissipation spectrum $15\nu k^2 E(k)$.

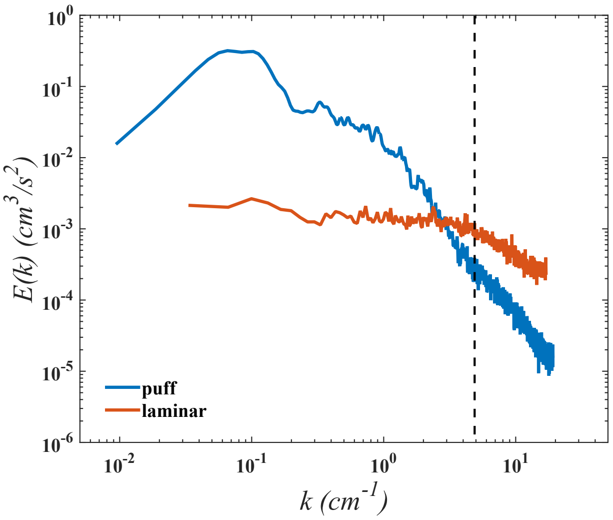


Figure S-13: Example of noise in $E(k)$ (from laminar flow) alongside $E(k)$ from a puff flow at the same $Re$, $Re = 2110$. For the laminar flow, the $E(k)$ at high $k$ is not flat (corresponding to noise spectrum). This high $k$ region is not trustworthy because it is influenced by the intermittent sampling time of the LDV at these higher wavenumbers (frequencies) [11, 12]. The dashed line shows the cutoff $k$, which we determined from $E(k)$ for the puff flow. The cutoff $k$ coincides with the $k$ where the $E(k)$ for laminar flow becomes untrustworthy.

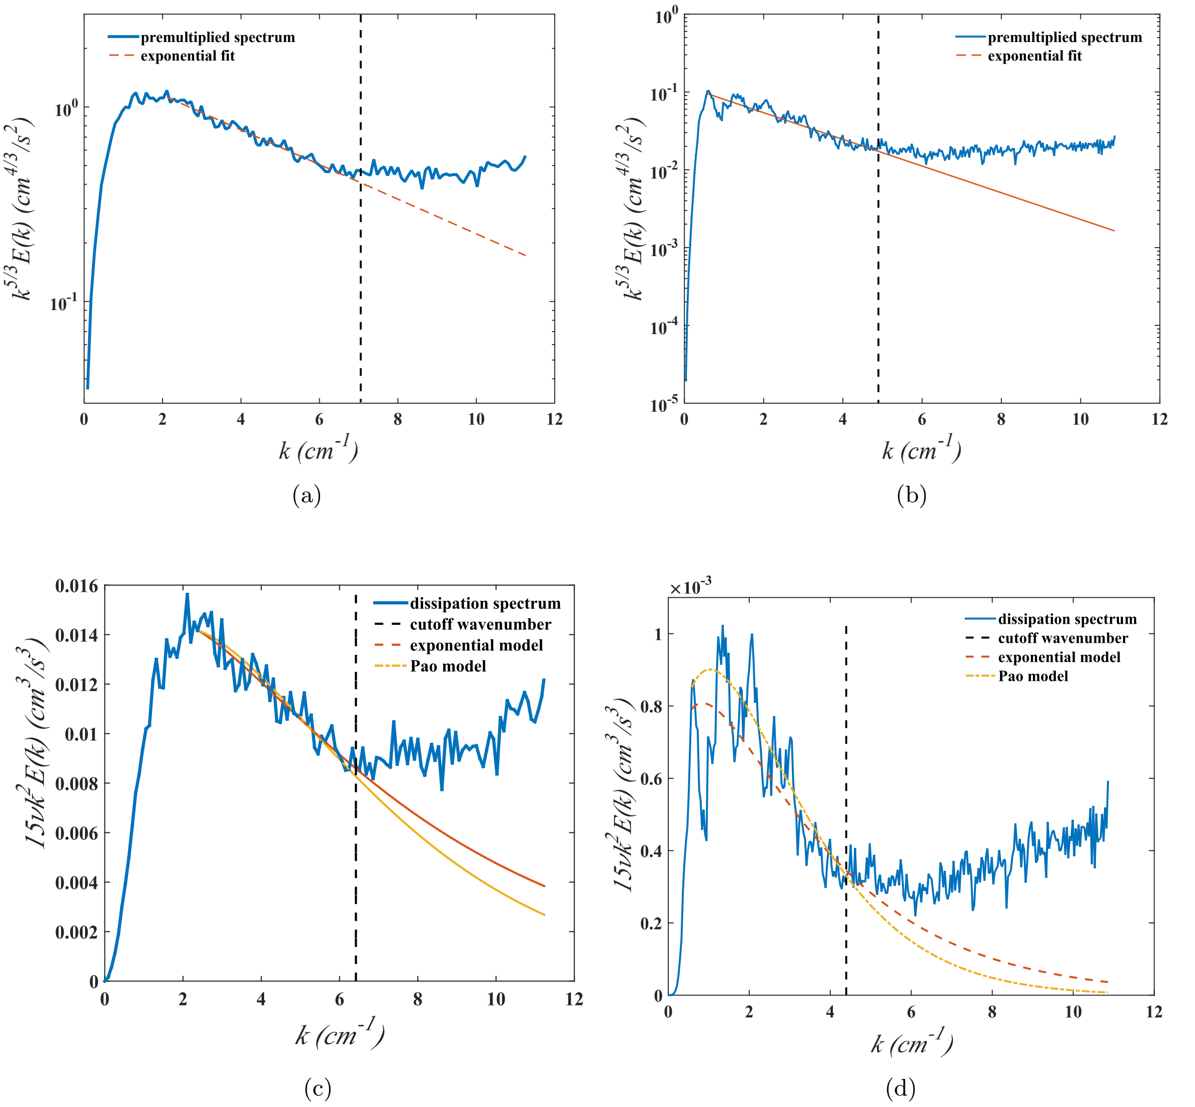


Figure S-14: (a,b) Premultiplied spectrum $k^{5/3}E(k)$ for turbulent flow at $Re = 12300$ (a) and for puff flow at $Re = 2350$ (b). The vertical dashed line marks the cutoff $k$ and the red dashed line shows the fit for the dissipation range with the exponential model. Each spectra is individually fit. (c,d) The dissipation spectrum $15\nu k^2 E(k)$ corresponding to panels (a) and (b), respectively. The dashed lines show the cutoff $k$, the exponential model, and the Pao model. Computing $\eta$ with and without extending the dissipation spectrum yields values within 2.5%.

From the dissipation spectrum, we compute $\eta$ (see Methods). In Fig. S-15 we plot $\eta/D$ vs. $Re$, where, in computing $\eta$, we have (1) extended $E(k)$ using the exponential model, (2) extended $E(k)$ using the Pao model, and (3) simply chopped off $E(k)$ at the cutoff $k$. Any of the three options does not not significantly alter the value of $\eta$, and we arrive at the same conclusion: $\eta/D \propto Re^{-3/4}$. Thus, Kolmogorov turbulence rules Reynolds's flashes.

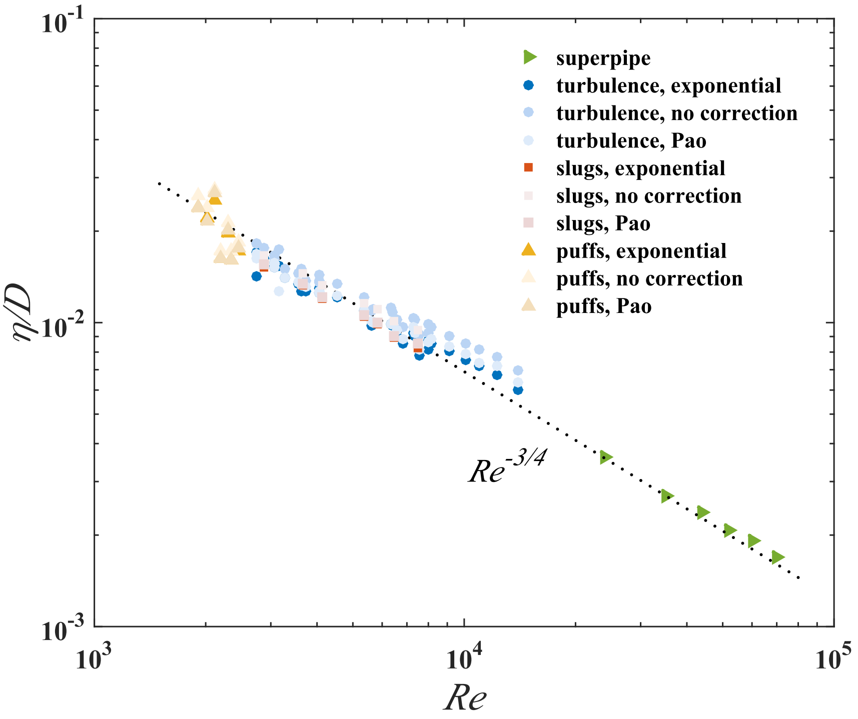


Figure S-15: $\eta/D$ vs. $Re$ for puff flows, slug flows, and turbulent flows. Various ways of computing $\eta$ yield the same conclusion: $\eta/D \propto Re^{-3/4}$.

In the plot of $\eta/D$ vs. $Re$ in the manuscript (Fig. 3c), we show error bars. We determine the vertical error bars for $\eta/D$ by the goodness of the fit of the exponential model to the premultiplied spectrum as well as the noise level in the LDV, as determined by the standard deviation of the laminar flow at the same $Re$ (see Fig. S-13). We determine the horizontal error bars for $Re$ based on the uncertainty from the flowmeter and statistical fluctuations of the flow itself. All horizontal error bars are too small to see but the vertical error bars are visible for puff flows.

# References


[1] K. Avila, D. Moxey, A. de Lozar, M. Avila, D. Barkley, and B. Hof, "The onset of turbulence in pipe flow," *Science*, vol. 333, no. 6039, pp. 192–196, 2011.

[2] T. Mullin, "Experimental studies of transition to turbulence in a pipe," *Annu. Rev. Fluid Mech.*, vol. 43, pp. 1–24, 2011.

[3] K. P. Nolan and T. A. Zaki, "Conditional sampling of transitional boundary layers in pressure gradients," *J. Fluid Mech.*, vol. 728, pp. 306–339, 2013.

[4] M. Sano and K. Tamai, "A universal transition to turbulence in channel flow," *Nature Phys.*, vol. 12, no. 3, pp. 249–253, 2016.

[5] G. Lemoult, L. Shi, K. Avila, S. V. Jalikop, M. Avila, and B. Hof, "Directed percolation phase transition to sustained turbulence in couette flow," *Nature Phys.*, vol. 12, no. 3, pp. 254–258, 2016.

[6] K. Avila and B. Hof, "High-precision taylor-couette experiment to study subcritical transitions and the role of boundary conditions and size effects," *Rev. Sci. Instrum.*, vol. 84, no. 6, p. 065106, 2013.

[7] M. Avila and B. Hof, "Nature of laminar-turbulence intermittency in shear flows," *Phys. Rev. E*, vol. 87, no. 6, p. 063012, 2013.

[8] D. Moxey and D. Barkley, "Distinct large-scale turbulent-laminar states in transitional pipe flow," *P. Nat. Acad. Sci. USA*, vol. 107, no. 18, pp. 8091–8096, 2010.

[9] S. Smith, *Digital signal processing: a practical guide for engineers and scientists.* Newnes, 2013.

[10] S. B. Pope, *Turbulent flows.* Cambridge University Press, 2000.

[11] H.-E. Albrecht, N. Damaschke, M. Borys, and C. Tropea, *Laser Doppler and phase Doppler measurement techniques.* Springer Science & Business Media, 2013.

[12] R. Adrian and C. Yao, "Power spectra of fluid velocities measured by laser Doppler velocimetry," *Exp. Fluids*, vol. 5, no. 1, pp. 17–28, 1986.

[13] O. Reynolds, "An experimental investigation of the circumstances which determine whether the motion of water shall be direct or sinuous, and of the law of resistance in parallel channels.," *P. Roy. Soc. Lond.*, vol. 35, no. 224-226, pp. 84–99, 1883.

[14] J. Den Toonder and F. Nieuwstadt, "Reynolds number effects in a turbulent pipe flow for low to moderate Re," *Phys. Fluids*, vol. 9, no. 11, pp. 3398–3409, 1997.

[15] S. G. Huisman, D. P. van Gils, and C. Sun, "Applying laser doppler anemometry inside a taylor–couette geometry using a ray-tracer to correct for curvature effects," *Eur. J. Mech. B-Fluid*, vol. 36, pp. 115–119, 2012.

[16] M. Nishi, B. Ünsal, F. Durst, and G. Biswas, "Laminar-to-turbulent transition of pipe flows through puffs and slugs," *J. Fluid Mech.*, vol. 614, pp. 425–446, 2008.

[17] D. Samanta, A. De Lozar, and B. Hof, "Experimental investigation of laminar turbulent intermittency in pipe flow," *J. Fluid Mech.*, vol. 681, pp. 193–204, 2011.
